# Supplementary material for: Unveiling Project-Specific Bias in Neural Code Models
Source: arXiv:2201.07381 source file (2024-03-11)
Supplement: Supplementary file 1 [file appendix.tex]

\section{Model Architectures}
\begin{itemize}[leftmargin=*]
    \item \textbf{CodeBERT}: The CodeBERT model uses the same model architecture as RoBERTa-base~\cite{zhuang2021robustly}, which consists of 6 layers, 768 dimensional hidden states and 12 attention heads. The total number of model parameters is 125M. The model is pre-trained on a dataset~\cite{husain2019codesearchnet} that contains bimodal datapoint: code function with paired documentation. The dataset includes 2.1M bimodal datapoints and 6.4M unimodal code across six programming languages (Python, Java, JavaScript, PHP, Ruby, and Go). The pre-training objectives of the CodeBERT model includes masked language modeling (MLM)~\cite{devlin2018bert} and Replaced Token Detection (RTD)~\cite{DBLP:conf/iclr/ClarkLLM20}.
    \item \textbf{GraphCodeBERT}: The GraphCodeBERT model uses the same model architecture as the CodeBERT model. It is pre-trained with the same dataset as CodeBERT. GraphCodeBERT is the first pre-trained model that leverages code structure to learn code representation to improve code understanding. It introduce a graph guided masked attention function to incorporate the code structure into Transformer and two new structure-aware pre-training tasks to learn representation from source code and code structure.
\end{itemize}

\section{Baseline Details}
\begin{itemize}[leftmargin=*]
  \item \textbf{Reweighting}: 
  This method first trains a bias-only model using recognized bias. Empirically, the bias-only model is often confident about its prediction and assigns high probability to samples with bias. Given with the confidence predicted by the bias-only model $p_{b}^{i}$, to train a de-biaed model, the classification loss of each training loss is reweighted with $1-p_{b}^{i}$ so that samples that exhibit bias are expected to be downweighted. Formally:
  \begin{equation}
      \mathcal{L}_\mathrm{DEBIAS}=-\mathbb{E}_{(x_i, x_j) \sim D}\left(1-p_{b}^{i}\right) y^{i} \cdot \log p_{d}^{i}
  \end{equation}
  where $p_{d}$ is the normalized predicted probability distribution of the debiased model. Specifically, in our implementation, for vulnerability detection, the bias-only model is trained on user-define variable and function names as well as macro-definitions; for type inference, the bias-only model is trained merely on the declaration variable representation. We use the CodeBert architecture for the bias-only model, which is the same as the debiased model.
  \item \textbf{Product-of-expert (PoE)}: Similarly to re-weighting, PoE also requires a trained bias-only model. The debiased model is trained in an ensemble manner with the bias-only model by combining their normalized prediction probability, which is as follows:
  \begin{equation}
      \mathcal{L}_\mathrm{DEBIAS}=-\mathbb{E}_{(x_i, y_i) \sim D}y^{i} \cdot \log \operatorname{softmax}[\log (p_{d}^{i} \cdot p_{b}^{i})]
  \end{equation}
  For PoE, the biased models we used are the same as those used in reweighting.
  
  \item \textbf{Adversarial training}: 
  Instead of updating the model with only original samples, adversarial training\cite{madry2017towards,goodfellow2014explaining} proposes to train the model with perturbed adversarial samples along with the original ones so that the model is expected to perform robustly when handling data with perturbations. Formally:
  \begin{equation}
      \mathcal{L}_\mathrm{DEBIAS}=-\mathbb{E}_{(x_i, x_i', y_i) \sim D} \mathcal{L}(x_i, y_i) + \mathcal{L}(x_i', y_i)
  \end{equation}
  where $x_{i}'$ is a perturbed version of the original sample $x$. In our implementation, we follow Yefet~\etal\cite{yefet2020adversarial} to perturb samples with non-targeted attack using single BFS step on the recognized bias tokens.
  
  \item \textbf{Gradient Reversal}:
  The methods propose to unlearn bias information explicitly in a minimax game manner. Specifically, it employs an additional bias prediction network $h$ to predict the bias distribution along with the standard target classification loss and update the weights of the backbone model adversarially by reversing the gradient of the bias prediction network so that at the end of training, the bias prediction network is unable to predict bias, since the backbone model $f$ has successfully unlearned the bias. Formally:
  \begin{equation}
  \begin{aligned}
      \min _{\theta_{f}, \theta_{g}} \max _{\theta_{h}}&\mathbb{E}_{(x_i, y_i) \sim D} \mathcal{L}(x_i, y_i;\theta_{f}, \theta_{g}) \\ &- \mu\mathcal{L}(b(x_i), h\circ f(x_i; \theta_{f},\theta_{h}))
  \end{aligned}
  \end{equation}
  where $g$ is the classification head layer for the regular target classification, $b(x_i)$ is the known bias of a sample $x_i$, in our case, it is the bias vocabulary set, $\mu$ is a regulatory coefficient which is set as 0.1 in our implementation.
  
\end{itemize}

\section{Ablation analysis}
\begin{figure*}[t]
\centering     %%% not \center
\subfigure{\label{fig:vd_abl_cb}\includegraphics[width=0.245\textwidth]{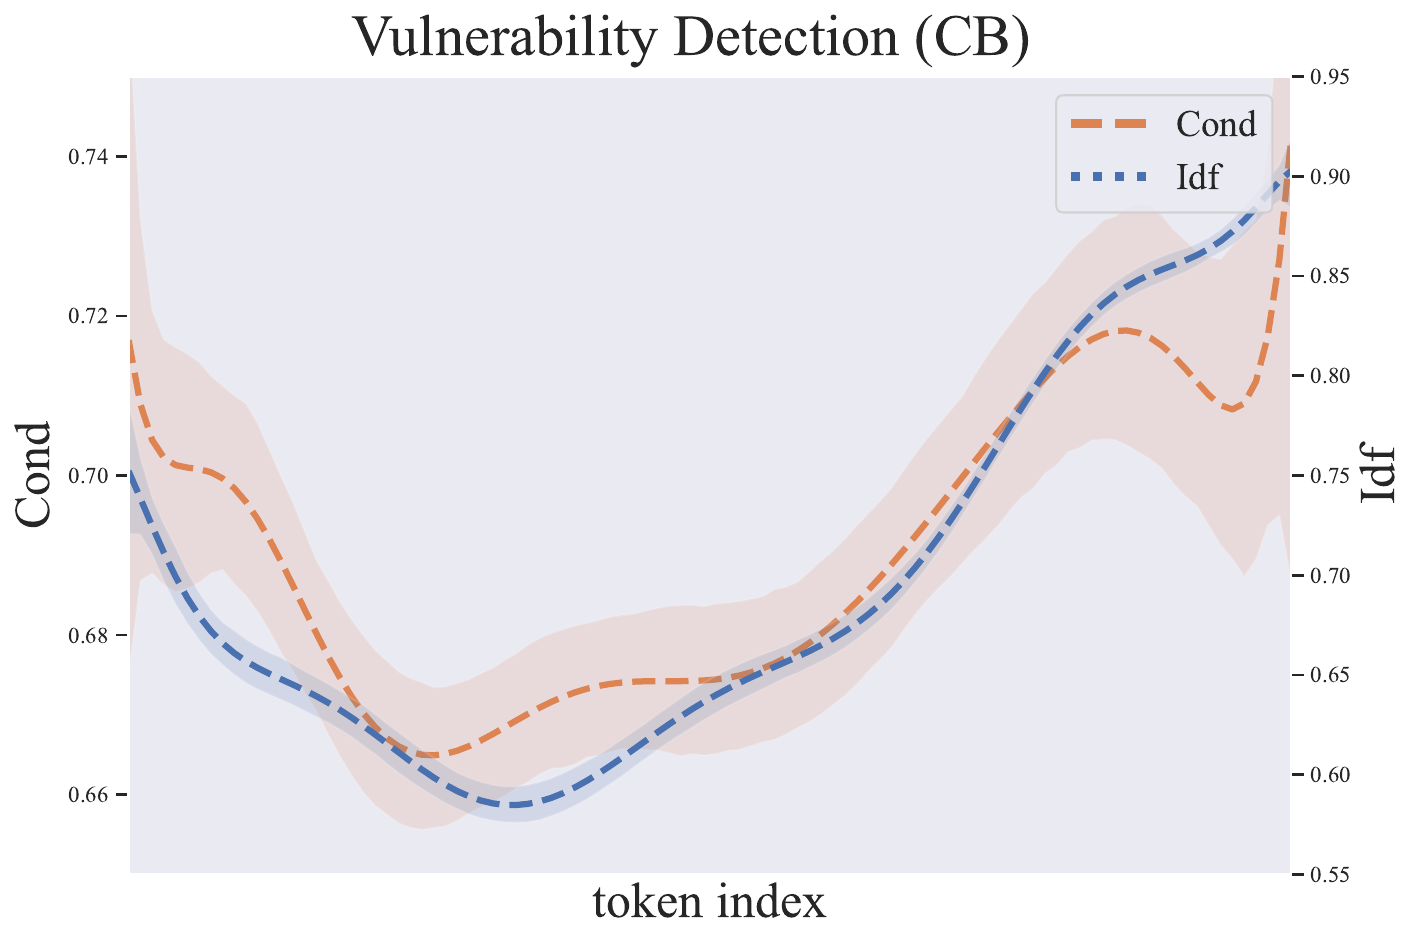}}
\subfigure{\label{fig:vd_abl_gcb}\includegraphics[width=0.245\textwidth]{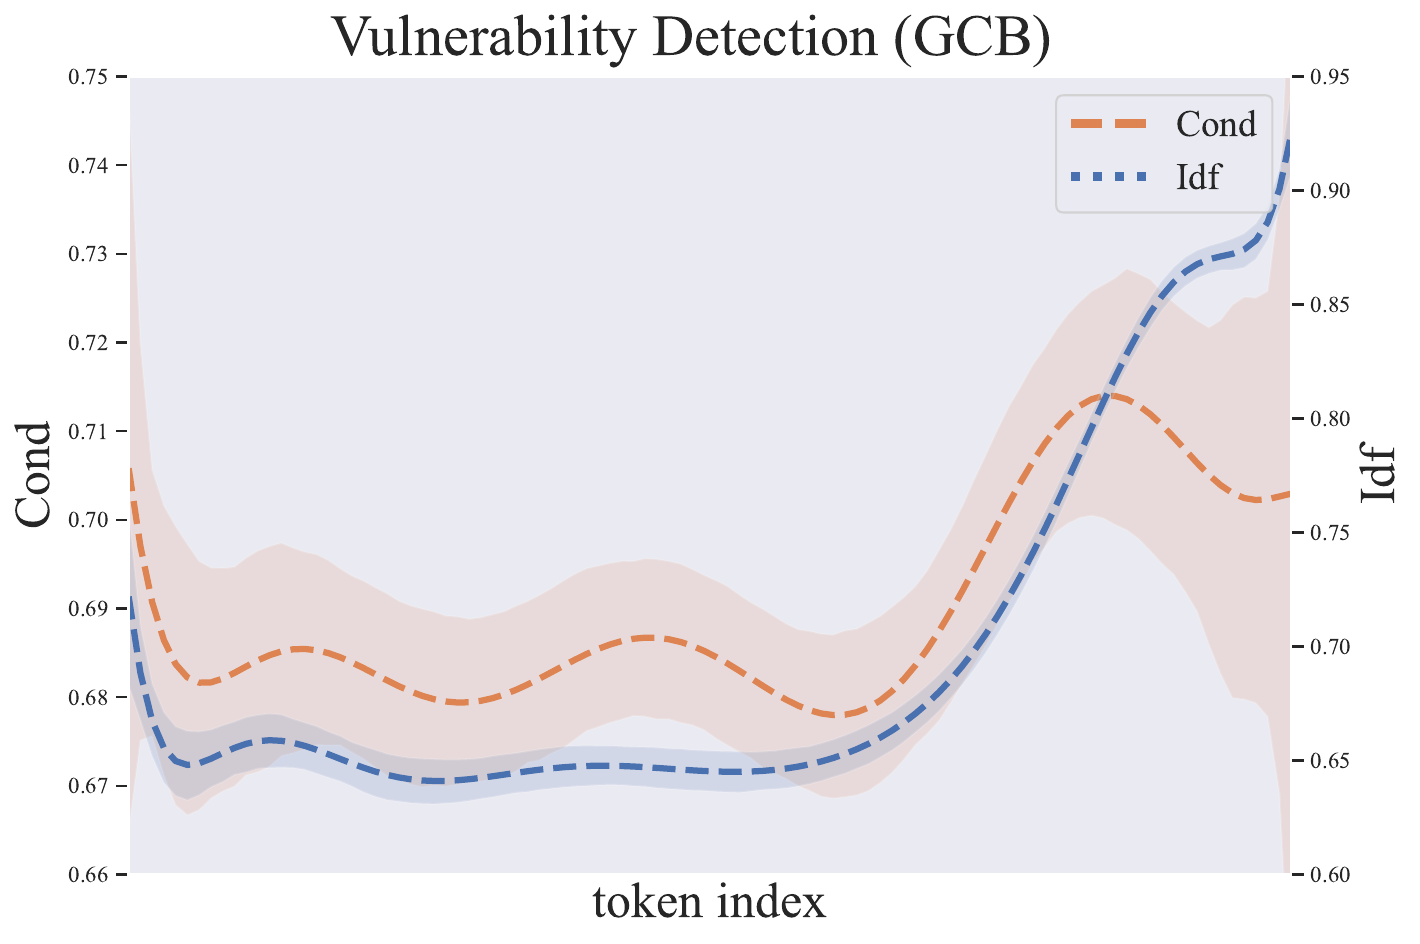}}
\subfigure{\label{fig:ti_abl_cb}\includegraphics[width=0.245\textwidth]{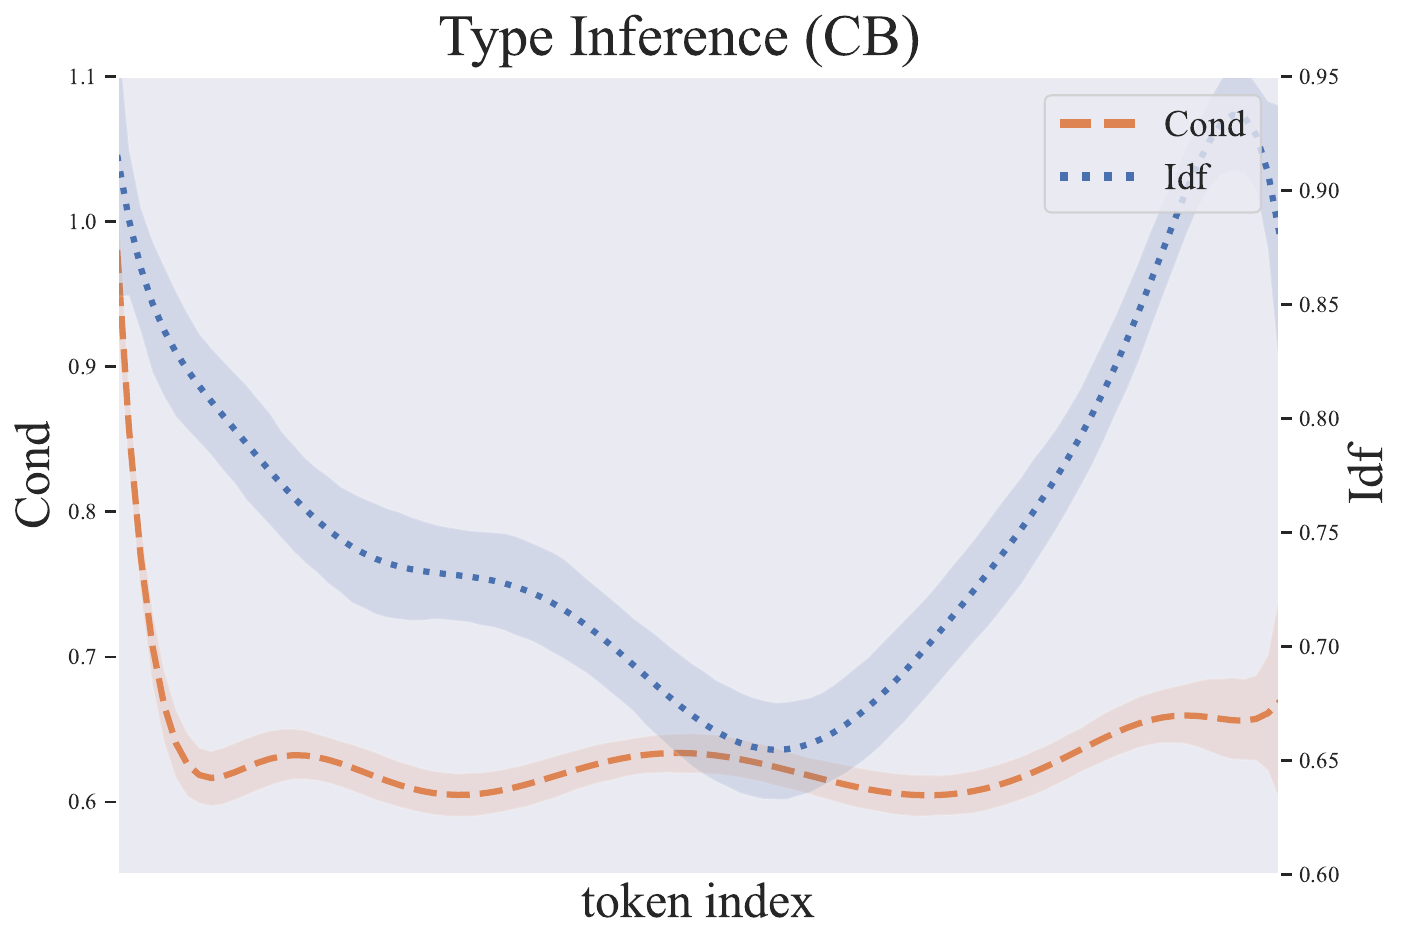}}
\subfigure{\label{fig:ti_abl_gcb}\includegraphics[width=0.245\textwidth]{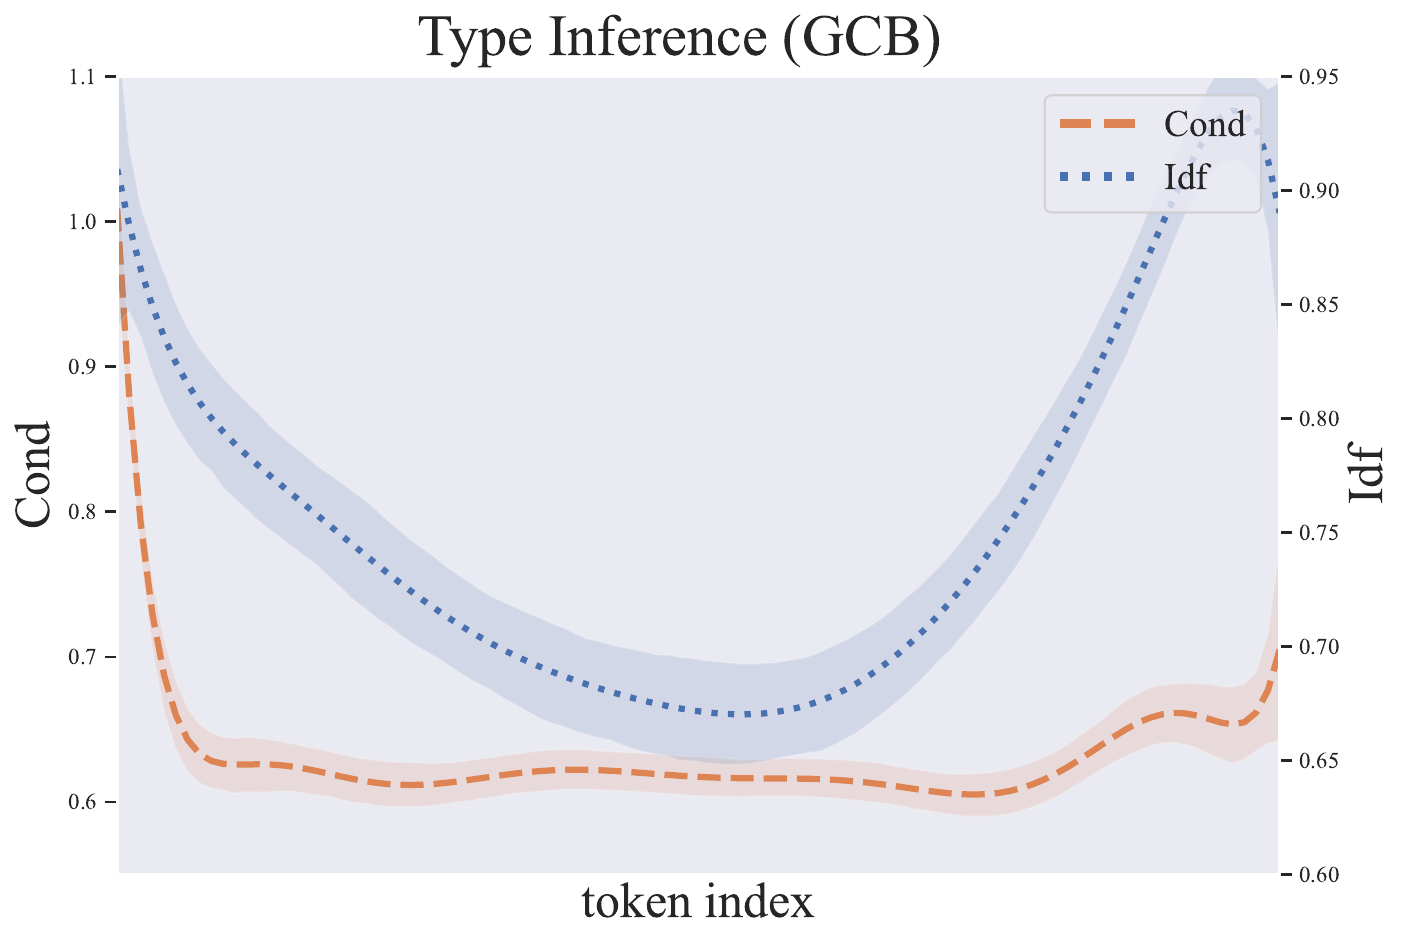}}\\

% \squeezeup
 \caption{The ablation analysis of the Cond-Idf measurement.}
\label{fig:bd}
\end{figure*}

In this section, we conduct an ablation analysis on the proposed Cond-Idf measurement. Specifically, we break the measurement into the conditional probability distribution approximation (Cond) and Idf distribution approximation. The results are shown in \Cref{fig:bd}. 

For the two evaluated models on both the vulnerability detection and type inference tasks, we can observe that the head of the ranked integrated gradient distribution positively correlates with both the Cond and Idf distributions. Quantitatively, to calculate the correlation, we sample 50 data points that are evenly spaced from the top 50\% of both the ranked integrated gradient distribution and the Cond/Idf distributions. We use the Spearman’s rank correlation as the measurement. \Eg~for the GCB model on the type inference task, the head of the Cond measurement and the ranked integrated gradient distribution are correlated with a Spearman's rank correlation of $\rho_\mathrm{{Cond}}=0.566$; and for the Idf measurement: $\rho_\mathrm{{Idf}} =1.00$. Similarly, for the CB model on the vulnerability detection task, the two measurements correlate with the ranked integrated gradient distribution with high rank correlation ($\rho_\mathrm{{Cond}}=0.561$, $\rho_\mathrm{{Idf}} =0.700$).  

% While for the GCB model, as shown in the figure, the correlation is lowered and the approximation curve is much more curly ($\rho_\mathrm{{Cond}}=0.504$, $\rho_\mathrm{{Idf}} =0.398$). We think this is because the the data-flow aware pre-raining objectives of the GCB model allow it to be less biased than the CB model thus making it less correlated with the Cond-Idf measurement.
